# Supplementary material for: FusionAI: Decentralized Training and Deploying LLMs with Massive Consumer-Level GPUs
Source: arXiv:2309.01172 source file (2023-09-03)
Supplement: Supplementary file 1 [file appendix.tex]

\newpage
\appendix
\section{Appendices}
\subsection{Additional Related Work}
\paragraph{Large Language Models} \label{sec:appllm}

Large-scale pre-trained models (LLMs) underpin advancements in computer vision (CV), natural language processing (NLP), and graph learning~\cite{zhou2023comprehensive}. In CV, models like the Vision Transformer (ViT) excel in image classification~\cite{dosovitskiy2020image}, SegAnything in semantic segmentation~\cite{kirillov2023segment}, DALL-E2 in generating images from text~\cite{DALL-E2}, and Stable Diffusion Models in image denoising and inpainting~\cite{stableDiffusion}. NLP has been revolutionized by LLMs like BERT for text classification and fine-tuning~\cite{devlin2018bert}, GPT series for text generation and language understanding~\cite{gpt,gpt2,gpt3,openai2023gpt4}, and ChatGPT for conversational context~\cite{chatgpt}. Graph learning has benefited from Graph Neural Networks (GNNs) and Graph Transformer Networks (GTNs) for various tasks like node classification and knowledge graph completion~\cite{kipf2016semi,chen2020simple}, and the Graph Attention Network (GAT) for aggregating neighboring information~\cite{velickovic2017graph}.

\paragraph{3D Parallelism}\label{sec:app3D}
Distributed training and inference can be categorized into data parallelism (DP), tensor parallelism (TP), and pipeline parallelism (PP). DP is a widely used technique in deep learning that distributes the training process across multiple devices or machines by dividing the training data into smaller subsets. These subsets are processed in parallel~\cite{tang2020communication}. The gradients or model parameters resulting from each subset are then aggregated and used to update the overall model parameters. This method facilitates faster and more efficient training of large neural networks.

However, DP faces challenges when accommodating large-scale LLMs within a single GPU due to limited GPU memory. TP and PP offer effective solutions to address this challenge. TP distributes the model across GPUs by partitioning tensors horizontally or vertically, while PP divides the model's layers into several stages. Each stage performs a forward pass to compute the activations for its layers and then passes these activations to the next stage.

Several existing LLM pretraining frameworks, including Transformers \cite{huggingface}, Megatron-LM \cite{mega1,mega2}, DeepSpeed \cite{deepspeed1}, and Colossal-AI \cite{colossal}, utilize model parallelism to pretrain LLMs. These frameworks distribute self-attention heads and feed-forward layers across multiple GPUs and transformer layers across multiple nodes, significantly reducing the memory load on individual GPUs. In addition, to ensure accurate forward and backward passes, these frameworks synchronize the parameters via communication operations such as reduce-scatter and all-gather \cite{mega1}.

While centralized 3D parallel training methods standardize the model partitioning process across nodes, heterogeneous hardware platforms introduce complexities to the model partitioning and communication due to their varied capabilities. Therefore, achieving parallelism on such platforms necessitates a thorough understanding of these differences, which we will illustrate in Section \ref{sec:decentralized}.

\subsection{Edge DL: Opportunities and Challenges}
% 1. This section provide related works about the edge DL
% 2. how our systems incorporate edge DL.

Compared to cloud servers, edge devices typically have limited resources in terms of memory, computational power, and energy, as well as restricted scalability. In order to accommodate these resource constraints, DNNs must be compressed. DNNs often exhibit a high degree of redundancy, and as a result, many existing approaches focus on minimizing this redundancy to strike an optimal balance between resource usage and model accuracy. One prevalent technique is low-precision inference Binaryconnect~\cite{courbariaux2016binaryconnect}, Lq-net~\cite{ZhangYangYeECCV2018} and Xnor-net~\cite{rastegari2016xnornet}, which involves quantizing weights into a lower bitwidth to enable more efficient operations and reduced storage requirements. While this method is necessary for deploying an entire model on an edge device, yet we do not force to do so even quantization can still maintain model performance.

To achieve memory-efficient and data-efficient on-device learning, several existing methods have been proposed, such as low-precision training \cite{NEURIPS2018_335d3d1c} \cite{cambier2020shifted} and trading memory for computation \cite{gruslys2016memoryefficient} \cite{chen2016training}. However, these techniques are primarily designed for high-throughput cloud training on large-scale datasets and may not be suitable for on-device learning with only a small number of data samples. Our work aims to harness the power of large-scale datasets for edge training by partitioning the workload into multiple workflows, offering scalability that adapts to the size of the device topology.

In addition to standalone edge devices, edge-server systems are another common infrastructure for edge intelligence applications. However, resources on edge devices are often limited, including memory, computing power, and energy, and wireless communication can also be constrained, such as limited bandwidth. An efficient updating and learning process that meets these constraints is necessary. Communication-efficient federated learning \cite{kairouz2021advances} \cite{lin2020deep} \cite{li2020lotteryfl} investigates methods for compressing multiple gradients (to be sent to the server) calculated on different sets of non-local data, enabling the aggregated compressed gradients to achieve similar convergence performance as centralized training on all data. To harness the power of numerous consumer devices while minimizing latency, our work implements a decentralized network architecture that allows for dynamic device connections and disconnections, along with automatic workflow assignments.

%  ====================== Leave for Arxiv and INFOCOM.... ====================== 
% \subsection{Distributed Optimization}\label{sec:DistOpt}
% In this paper, we differ distributed optimization from the distributed training. The distributed training mainly refers to the ways how datasets, hidden features, models and gradients are allocated, and how computing are scheduled to implement efficient pipeline. And the distributed optimization mainly means how to use distributed gradients to update model parameters. In our system..................

\subsection{Incentive Mechanism}\label{sec:incentive}
% The incentive mechanism in decentralized scientific computing refers to the rule and system to achieve desired performance in situations where multiple self-interested individuals interact. The main objective of the incentive mechanism is to create mechanisms that are incentive-compatible, meaning they encourage participants to truthfully reveal their preferences and engage in contributing their resources(e.g., computational power or storage space) that maximize performance. This is often done through the use of incentives, such as rewards or penalties(e.g., direct payments or access to exclusive content or services), to align individual interests with collective goals.

% The incentive issues are vital to decentralized scientific computing. decentralized scientific computing mainly consumes computation power and bandwidth from participants,  some of which might be constraint in scenarios like mobile networks and mobile edge computing.

%  ----------- Incentive Mechanism. ----------
Incentive mechanism is a economic catalyst to make decentralized training become a reality. Some previous schemes like auction, contract, Stackelberg game, etc. can be employed to incentivize some selfish and rational clients to participate this cooperative learning. Compared with previous incentive schemes in other similar scenarios, there are some special challenges and considerations in the mechanisms design. (1) The property of online training indicates that the arrival and departure time is unknown and varies drastically for different clients. This online property is in line with asynchronous training but malfunctions previous one-round incentive schemes. (2) Some other alternative choices should be considered for clients like bitcoin mining, client-assisted contributions, etc.,  which can also bring some economical benefits to their participation. In other words, incentive design should attracts clients to join in decentralized learning from many candidate choices. (3) The incentive scheme should be robust and resilient to some malicious clients which contribute nothing but endeavor to get large paybacks. 
 
% ------------ Relation between Incentive Mechanism and our system ------------
In our system..................

\subsection{Security}\label{sec:security}

The security challenges in decentralized computing are also a critical concern. The potential for data privacy infringement due to the risk of unauthorized data access and manipulation~\cite{li2022enigma}\cite{hitaj2017deep}\cite{zhu2019deep}. There is also the threat of malicious computing nodes that can disrupt system operations and compromise model robustness~\cite{bagdasaryan2020backdoor}. The issue of Membership Inference  can expose if a specific data point was used in training the model~\cite{shokri2017membership} \cite{nasr2019comprehensive}. In response to these challenges, privacy-preserving techniques such as Secure Multiparty Computation (SMC), Differential Privacy, and Encryption are suggested as mitigation strategies~\cite{araki2016high} \cite{geyer2017differentially}\cite{{li2020invisiblefl}.

decentralized system

% ------------ Relation between decentralized system and our system ------------
In our system..................

\subsection{Hardware Performance Modeling}\label{sec:PerfModel}
In our work, it is important to accurately predict the computation and communication time of neural modules. Based on the accurate hardware performance modeling, the load balance scheduling can work better to alleviate the waiting time of the fast devices. Thus, the total execution time can be reduced.

Works that predict the computation and communication time can be divided into the DNN-based and analytic performance model. The DNN-based methods~\cite{8622396} proposes to train a DL model to predict the execution time for a given DNN model. Such DNN-based model may need large overhead to train and storage, adding much more extra computation burden to the low computing ability node in our scenario. More crucially, the computing providers are dynamic and heterogeneous, making it difficult to adapt the learned performance model to the newly joined nodes. 

The analytic performance model estimates the hardware performance based on model sizes, communication bandwidth and latency, and FLOPS of GPUs and CPUs, etc. With a short period of profiling to fit few parameters, analytic performance models can approximate the hardware performance with small errors~\cite{qi2017paleo,park2020hetpipe}.

\subsection{Energy and Carbon Footprint}\label{sec:energy}
% The energy and carbon footprint of deep learning refers to the environmental impact of the computational resources required to train and run deep learning models. Deep learning models require massive amounts of computational power, which translates into high energy consumption and carbon emissions, primarily due to the use of data centers powered by non-renewable energy sources. The energy consumption of deep learning models can be reduced through various methods, such as optimizing model architecture, using specialized hardware like GPUs or TPUs, and implementing energy-efficient training algorithms. Additionally, the use of renewable energy sources, such as solar or wind power, can help reduce the carbon footprint of deep learning. The energy and carbon footprint of deep learning is a significant concern in the industry, and efforts are being made to develop sustainable and environmentally friendly deep learning practices.

% overview
energy consumption challenge:\cite{david_carbon2022}\cite{luccioni2022estimating}\cite{zhang2022opt}

%  ----------- Related works of energy and carbon footprint. ----------
energy optimization via power management: \cite{tang_dl2019}\cite{zeus_you_nsdi2023}\cite{cooperative_kang_tie2022}\cite{dynamic_wang_tpds2022}

energy optimization via adaptive batching and alignment: \cite{batch_dvfs_tpds2022}\cite{energy_wang_tgcn2022}

energy optimization via scheduling, including cloud-edge collaboration: 
\cite{know_yu_hpca2023}\cite{energy_wang_tpds2022}

% ------------ Relation between energy consumption and our system ------------
Currently, the energy consumption of high-end GPUs has become a bottleneck for training large models. In contrast, our proposd FusionAI can address this bottleneck by providing feasibility in terms of power consumption and offering more optimization opportunities and flexibility for energy efficiency. By leveraging existing relevant technologies discussed above, further improvements can be made to enhance global performance and energy efficiency.
